# Supplementary material for: Rank & Sort Loss for Object Detection and Instance Segmentation
Source: arXiv:2107.11669 source file (2021-08-30)
Supplement: Supplementary file 8 [file 8.Appendix.tex]

%\appendix
%\addcontentsline{toc}{section}{Appendices}
%\maketitle
\section*{APPENDICES}

%\begin{abstract}
%This document provides details for and supporting the material in the paper. 
%\end{abstract}
\renewcommand{\thefigure}{A.\arabic{figure}}
\renewcommand{\thetable}{A.\arabic{table}}
\renewcommand{\theequation}{A.\arabic{equation}}
%\pagebreak
\renewcommand{\thesection}{A}
\input{appendix/1.DetailsofRSLoss}
\renewcommand{\thesection}{B}
\input{appendix/2.Analysis}
\renewcommand{\thesection}{C}
\input{appendix/3.MoreExperiments}
%\bibliography{detectionbibliography_appendix}
